# Supplementary material for: Exploring What Why and How: A Multifaceted Benchmark for Causation Understanding of Video Anomaly
Source: arXiv:2412.07183 source file (2024-12-10)
Supplement: Supplementary file 1 [file X_suppl.tex]

\clearpage
\setcounter{page}{1}
% \maketitlesupplementary

\appendix
\setcounter{table}{0}

\setcounter{figure}{0}

% \begin{center}
% \noindent \textcolor{red}{Note: This document contains offensive content!}
% \end{center}

\section{Dataset}
\label{appendix a}
\subsection{Application of the proposed importance curve}

\begin{figure*}[h!]
    \centering
    \includegraphics[width=0.8\textwidth]{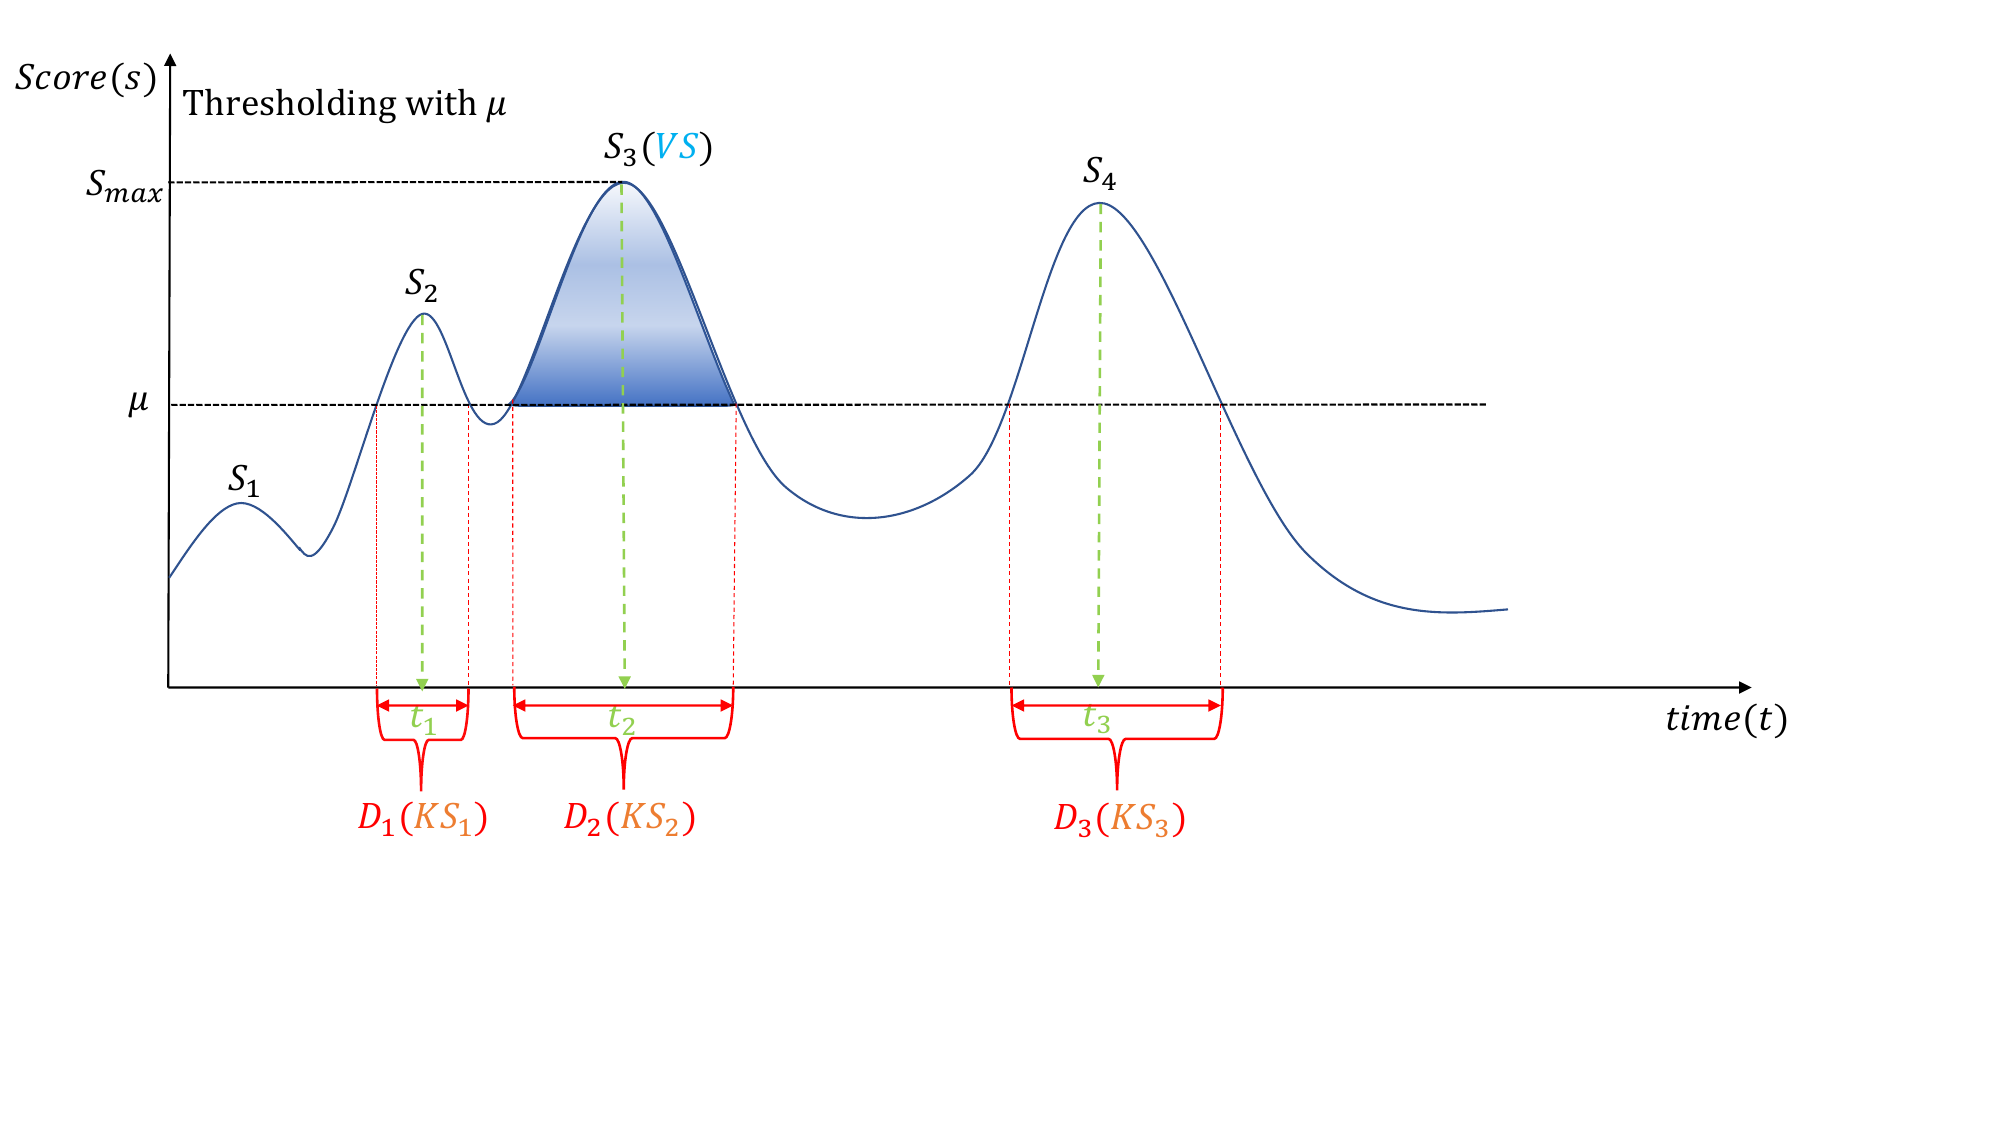}
    \caption{The application of the proposed importance curve, $KS_1$,$KS_2$ and $KS_3$ refer to three different key sentences. $VS$ point is the absolute maximum point in the curve. $t_1$, $t_2$, and $t_3$ are the timestamps of the local maximum point in the curve.}
    \label{fig:curve}
\end{figure*}
We have presented a novel annotation approach called the importance curve in section 3.1 of the main paper.
Such an approach enables us to unify various Video Temporal Grounding labels and tasks under the same framework.
Here, we describe how to apply the importance curve to unify various Video Temporal Grounding labels and tasks (e.g. Moment Retrieval, Highlight Detection, Video Summarization) respectively with Figure \ref{fig:curve}.\\
\textbf{Moment Retrieval} aims to retrieve time intervals from videos based on textual queries\cite{univtg}. 
The importance curve reflects the changing trends in the severity of anomaly. 
Thus, we first filter out the time intervals (e.g. $D_1$, $D_2$, and $D_3$ in Figure \ref{fig:curve}) through a threshold $\mu$.
Second, after post-processing the importance curve in Appendix A.4, we can obtain key sentences (e.g. $KS_1$, $KS_2$, and $KS_3$) corresponding to each time interval.
% And we annotate each time intervals with corresponding key sentences . 
% By applying a threshold $\mu$, we obtain the corresponding time intervals for key sentences.
Finally, these key sentences are employed as text queries, with corresponding time intervals serving as labels for the moment retrieval task. \\
\textbf{Highlight Detection} aims to assign a worthiness score to each video segment and then identify the top highest-scoring segment as the highlight \cite{univtg}. 
Here, we first locate the absolute maximum point of the curve (e.g. $VS$ in Figure \ref{fig:curve}), and leverage its corresponding time interval (e.g. $D_2$) as the top highest-scoring segment to conduct highlight detection task.\\
\textbf{Video Summarization} aims to summarize the whole video by a set of shots to provide a quick overview\cite{univtg}.
As depicted in Figure \ref{fig:curve}, $t_1$, $t_2$, and $t_3$ are the timestamps of the local maximum point (e.g. $S_2$, $S_3$ and $S_4$).
We leverage these timestamps as a set of shots to provide a quick overview of the whole video.
% \subsection{Downstream Task}

% \subsection{CUVA Dataset}
% We have shown the annotation pipeline of the proposed CUVA in the subsection $3.3$ of the main paper.  Here we provide a detailed description of our annotation process and present the comprehensive statistics of the dataset.\\
% \textbf{Annotation Process:}\\\\
\begin{figure*}[h!]
    \centering
    \includegraphics[width=1.0\textwidth]{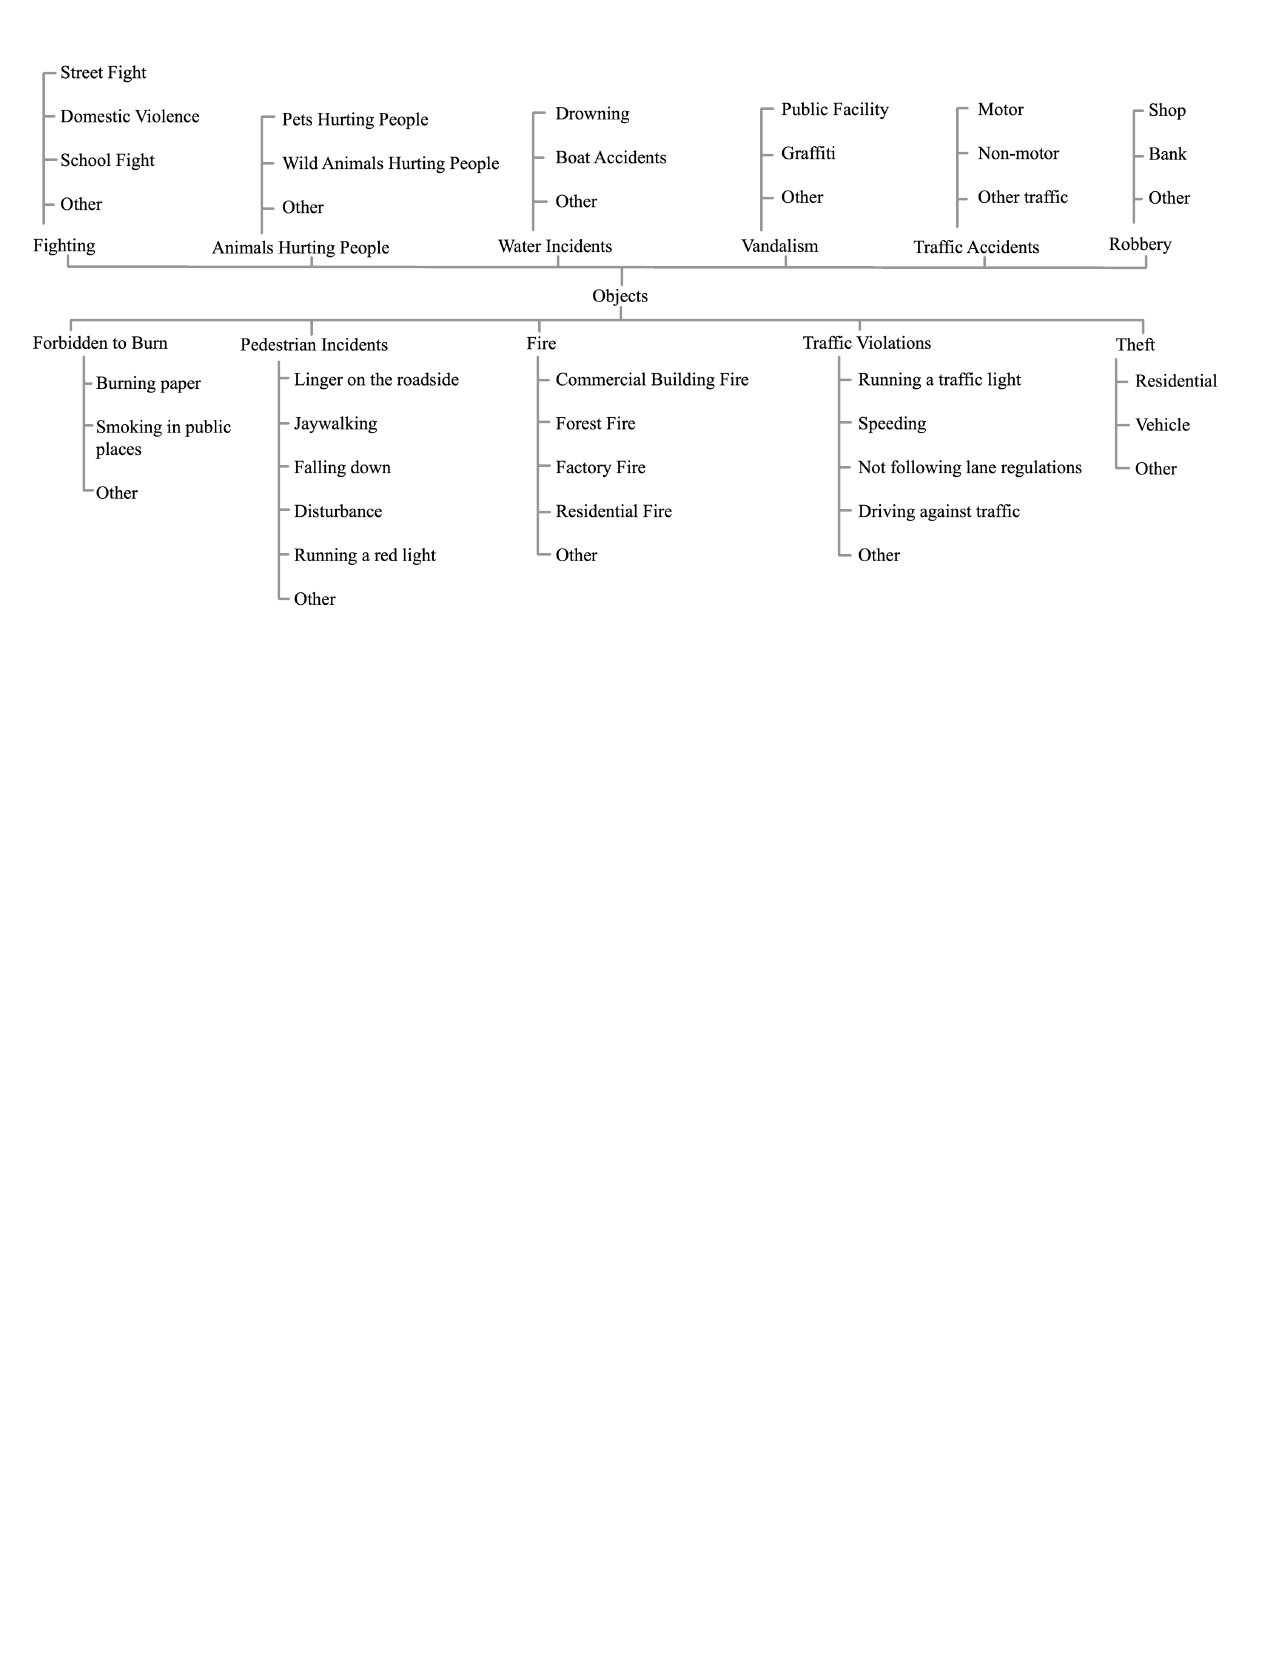}
    \caption{Anomaly types of the proposed CUVA, CUVA encompasses $11$ different scenes and $42$ extensive types of anomalies.}
    \label{fig:type}
\end{figure*}
\subsection{Our CUVA benchmark}
We have shown the statistics of the proposed CUVA in the subsection $3.5$ of the main paper.  
Here, we provide some supplementary for the statistics of the proposed CUVA.
As Figure \ref{fig:type} shows, we present more detailed statistics of video anomaly categories.
Figure \ref{fig:wordclouds} shows the word cloud of the proposed CUVA.
\begin{figure}[h!]
    \centering
\includegraphics[width=0.2\textwidth]{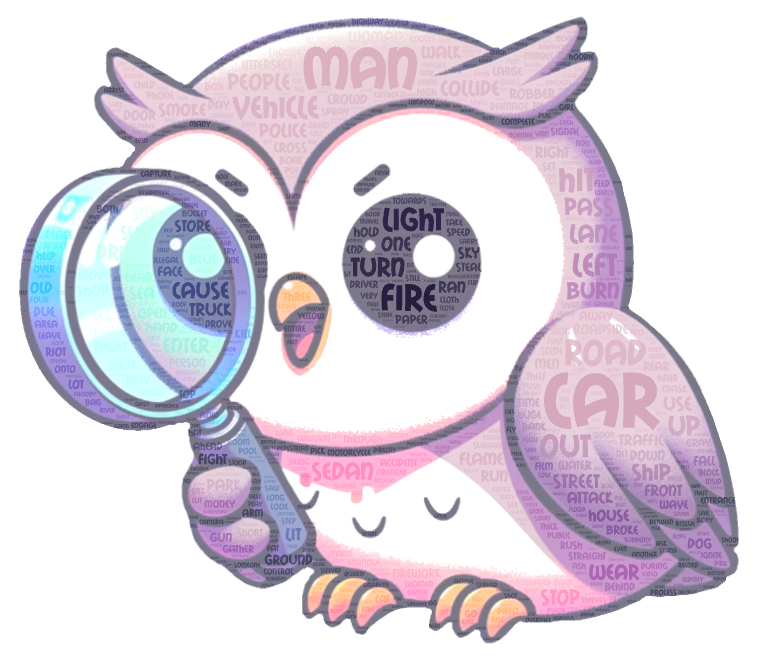}
    \caption{Wordcloud of our proposed CUVA.}
    \label{fig:wordclouds}
\end{figure}

\subsection{Ethical consideration}
\label{screening criteria}
We carefully study the online copyright rules of the websites from YouTube and Bilibili, from which we collect data, and strictly conform to their requirements during data collection and annotation. 
We have also adhered to the guidelines provided by the CVPR Code of Ethics to anonymize the parts of the video that may involve personal privacy by applying pixelation.
% We further request annotators pay attention to the protection of personal privacy while labeling, which can be found in subsection A.3.
% After the dataset is made public, we will develop an online agreement to require every user of the dataset strictly conform to the rules of the websites from which we collected the data.
To exclude data that could potentially have ethical implications. 
We further conduct rigorous reviews at each stage of the annotation, adhering to screening criteria as follows:\\

\begin{enumerate}[label=\arabic*.]
    \item \textbf{Personal Privacy Respect:}
        Avoid videos that show identifiable personal information (e.g., faces, license plates, home addresses).
    
    \item \textbf{Legally Sourced Content:}
        Prohibit the use of unauthorized or illegally obtained footage.
    
    \item \textbf{Viewer Sensitivity Consideration:}
        Avoid content that is overly graphic, cruel, or likely to cause viewer discomfort.
    
    \item \textbf{Child Safety Focus:}
        Exclude any videos involving children in risky or harmful situations.
    
    \item \textbf{Gender Respect and Equality:}
    \begin{itemize}
        \item Videos should not imply or display acts of sexual violence.
        \item Avoid content that contains gender discrimination or negative stereotypes of any gender group.
    \end{itemize}
    
    \item \textbf{Avoidance of Illegal Activities:}
   Do not display or promote videos that clearly show or endorse illegal activities (e.g., drug use, trafficking).
    
    \item \textbf{Copyright infringement:}
    Videos containing copyrighted music, film clips, TV shows, or other media content.
    
\end{enumerate}

% We provide examples of content that did not meet these criteria and were consequently removed from CUVA due to their offensive nature.

% \subsection{Ethical Consideration}
% We carefully study the online copyright rules of the websites from YouTube and Bilibili, from which we collected data, and strictly conformed to their requirements during data collection and annotation. 
% We have also adhered to the guidelines provided by the CVPR Code of Ethics to anonymize the parts of the video that may involve personal privacy by applying pixelation.
% We further request annotators pay attention to the protection of personal privacy while labeling, which can be found in subsection A.3.
% After the dataset is made public, we will develop an online agreement to require every user of the dataset strictly conform to the rules of the websites from which we collected the data.
\begin{figure}[h!]
    \centering
    \includegraphics[width=0.4\textwidth]{fig/postprocessing.pdf}
    \caption{Overview of the curve optimization pipeline}
    \label{fig:post_processing}
\end{figure}
\subsection{Post-processing of the importance curve}
As the initial sampling frequency of our curves is relatively lower (one frame per second), and we aim to obtain more accurate interval timestamps.\footnote{We leverage algorithm \ref{alg of curve} in the appendix to better illustrate the creation of the importance curve.}
Thus, we incorporate three specific tasks into our optimization strategy to achieve an optimal importance curve. 
% The original curve is derived following the annotation procedure in subsection 3.3.3 of the main paper.
Specifically, we perform tasks such as Video Captioning, Video Entailment, and Video Grounding by VideoChat\cite{2023videochat}, SEVILA\cite{sevila}, and UniVTG\cite{univtg}, respectively. 
Each task identifies specific time segments in the video based on the key sentences as shown in Figure 3 of the main paper. 
We adopt a voting mechanism to select a time segment when at least two models agree that it encapsulates the event represented by the key sentence annotation. 
Through the voting mechanism, we precisely identify the time segments in the video that correspond to the current key sentences. 
Then, we perform dense sampling on the voted segments (ten frames per second) and use wavelet filters to smooth the curve.
The comprehensive optimization process is illustrated in Figure \ref{fig:post_processing}.

\section{The proposed method}
\label{appendix b: method}
We have introduced A-Guardian, a novel prompt-based method that consists of two kinds of prompt design. 
Here, we detail the design of the hard prompts. 
Moreover, we illustrate the details of the answer prediction in this section.
\begin{figure*}[htbp]
    \centering
    \includegraphics[width=1\textwidth]{fig/hard_prompt-1-4.pdf}
    \caption{System message for VLMs. To guide the model for a description or answer, A-guardian uses different designed system messages for different tasks.}
    \label{fig:hard_prompt-1}
\end{figure*}
\subsection{Hard prompts in A-Guardian}
First, A-guardian leverages different newly designed system messages for different tasks, which can be found in Figure \ref{fig:hard_prompt-1}. 
After the VLM gives the answer based on the user message, the user's question and the VLM's answer will be input into ChatGPT to generate a new round of questions, 
Then, we re-input the question of ChatGPT\cite{chatgpt} into VLM, and the final answer will be obtained after several rounds of loops.
Figure \ref{fig:hard_prompt-2-1} and \ref{fig:hard_prompt-2-2} illustrate an A-Guardian hard prompt example which includes three rounds of dialog with ChatGPT.

\begin{figure*}[!h]
        \centering
    \includegraphics[width=1\textwidth]{fig/hard_prompt-1-2.pdf}
    \caption{An example of hard prompt in A-Guardian. After three rounds of dialog, the Video-ChatGPT model gives a more detailed, accurate, and focused description of the anomalous events in the video.}
    \label{fig:hard_prompt-2-2}
\end{figure*}
\begin{figure*}[!h]
    \centering
    \includegraphics[width=0.95\textwidth]{fig/hard_prompt-1-3.pdf}
    \caption{An example of Hard Prompts in A-Guardian (Extension of Figure \ref{fig:hard_prompt-2-2})}
    \label{fig:hard_prompt-2-1}
\end{figure*}
\subsection{Answer prediction}
We denote the candidate answers as $A$, we leverage BERT to generate the contextualized representations of each candidate answers $X_a$. 
We follow the previous work \cite{yang2021justask} to calculate the similarity between $X_k$ and the feature of all candidate answers $X_A = \{x_a | a \in A\}$ obtained by using the pre-trained model. 
Finally, the candidate answer with the maximal similarity is considered as the final prediction $\tilde{y}$. 
\begin{align}
    \tilde{y} = \arg\max_{y \in A} (X_k(X_A)^T)
\end{align}
During training, we optimize the softmax cross-entropy loss between the predicted similarity scores and ground truth.
\section{Experiment}
\subsection{Prompts of MMEval}
In MMEval, we have different scoring criteria for different tasks, which are translated into the system message of the VLM. Details can be found in Figure \ref{fig:mmeval_prompt}.
\begin{figure*}[htbp]
    \centering
    \includegraphics[width=1\textwidth]{fig/hard_prompt-1-1.pdf}
    \caption{System Messages for MMEval. In the design of the proposed MMEval metric, we apply different criteria for tasks involved in the proposed CUVA by different system messages, and the model is guided for scoring through different system messages.}
    \label{fig:mmeval_prompt}
\end{figure*}
\subsection{Case study of A-Guardian}
We have already shown the case study in section 5.6 of the main paper. 
Here, we further validate the effectiveness of the proposed model A-Guardian by the case study as follows:
Figure \ref{fig:case_study_appendix} shows the results from Video-ChatGPT with and without A-Guardian for the Description, Cause, and Effect tasks related to the same anomalous video. It can be observed that A-Guardian possesses the following abilities:
\begin{itemize}
    \item \textbf{Capturing key cues in the long video:} In the Description task, A-Guardian assists the VLM in identifying crucial moments and events in the anomalous video. For example, \textit{punching another man in the face} and \textit{holding a gun and pointing it at another man}. Whereas Video-ChatGPT without A-Guardian can only provide vague responses about the anomaly event.
    \item \textbf{Building a logic chain of cause and effect:} In the Cause and Effect tasks, A-Guardian guides the model in logical reasoning. In the example, the model with A-Guardian infers that the gun is the fundamental cause of the anomaly, leading to multiple injuries and people falling, followed by the perpetrator leaving. In contrast, the VLM without A-Guardian generates answers that are ambiguous and irrelevant to the events. The result emphasizes the potential results and societal impacts of the anomaly, lacking inference and summarization based on the video content.
 \end{itemize}
\begin{figure*}[htbp]
    \centering
    \includegraphics[width=1\textwidth]{fig/case_study_appendix.pdf}
    \caption{Case study of A-Guardian. We test the Video-ChatGPT model with and without the proposed A-Guardian. Equipped with A-Guardian, Video-ChatGPT can generate a more accurate and detailed description of the anomalies as well as reasonable causes and effects. In the Description task, VLM with A-Guaidian could generate \textit{punching another man in the face} and \textit{holding a gun and pointing it at another man}, whereas Video-ChatGPT without A-Guardian can only provide vague responses about the anomaly event, which proves that the proposed A-Guardian assists the VLM in capturing key cues in the long video. In the Cause task, the model with A-Guardian infers that the gun is the fundamental cause of the anomaly, leading to multiple injuries and people falling.}
    \label{fig:case_study_appendix}
\end{figure*}
\label{appendix c: method}
